# Supplementary material for: Forward-backward correlations with strange particles in PYTHIA
Source: arXiv:1510.02080 ancillary file (2015-10-07)
Supplement: Supplementary file 1 [file supplementary_plots_FB_Strangeness_in_PYTHIA_SQM2015.pdf]

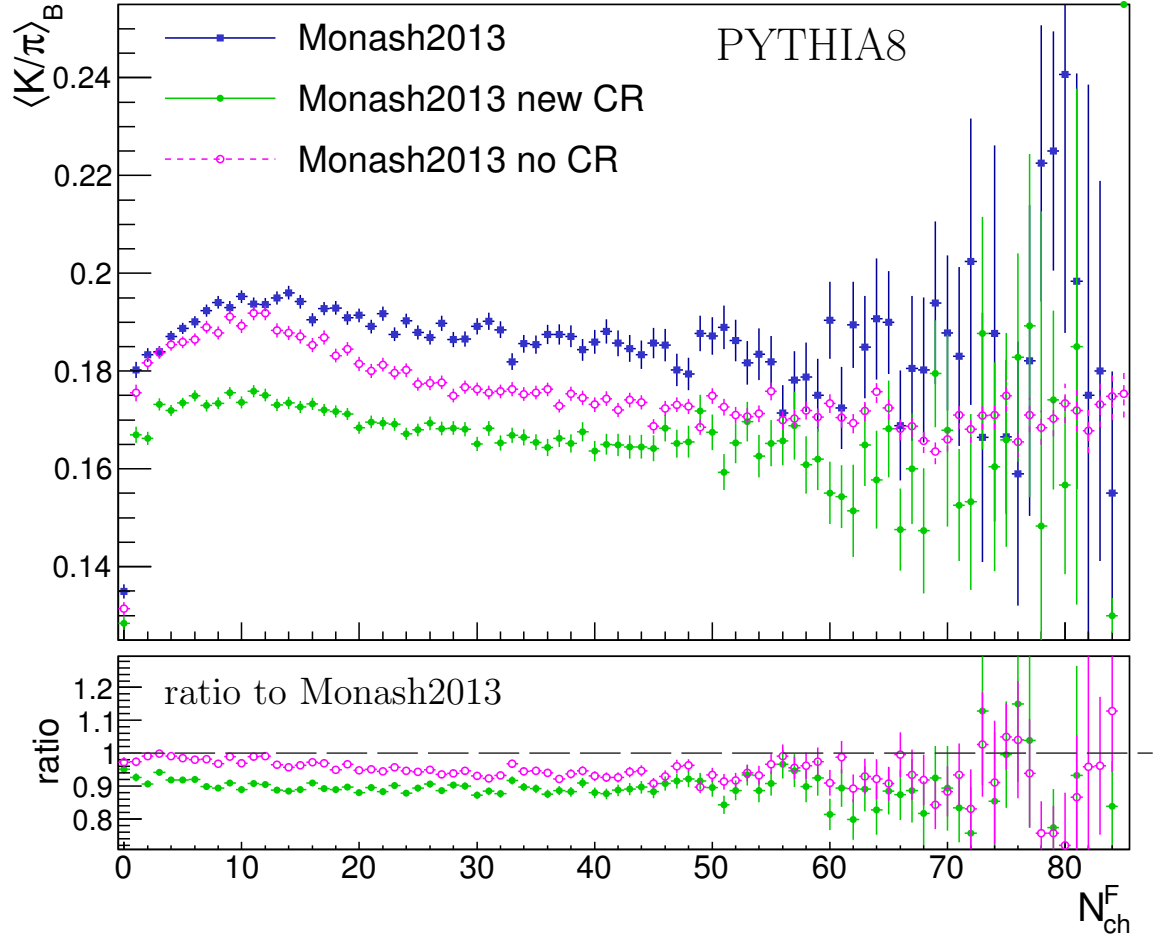

**Figure 1.** Forward-backward correlation between  $\langle K/\pi \rangle$  in backward window and  $N_{ch}$  in forward window, for three configurations of PYTHIA8 (version 8210). FB windows are  $-2.4 < \eta < -0.5$  and  $0.5 < \eta < 2.4$ .

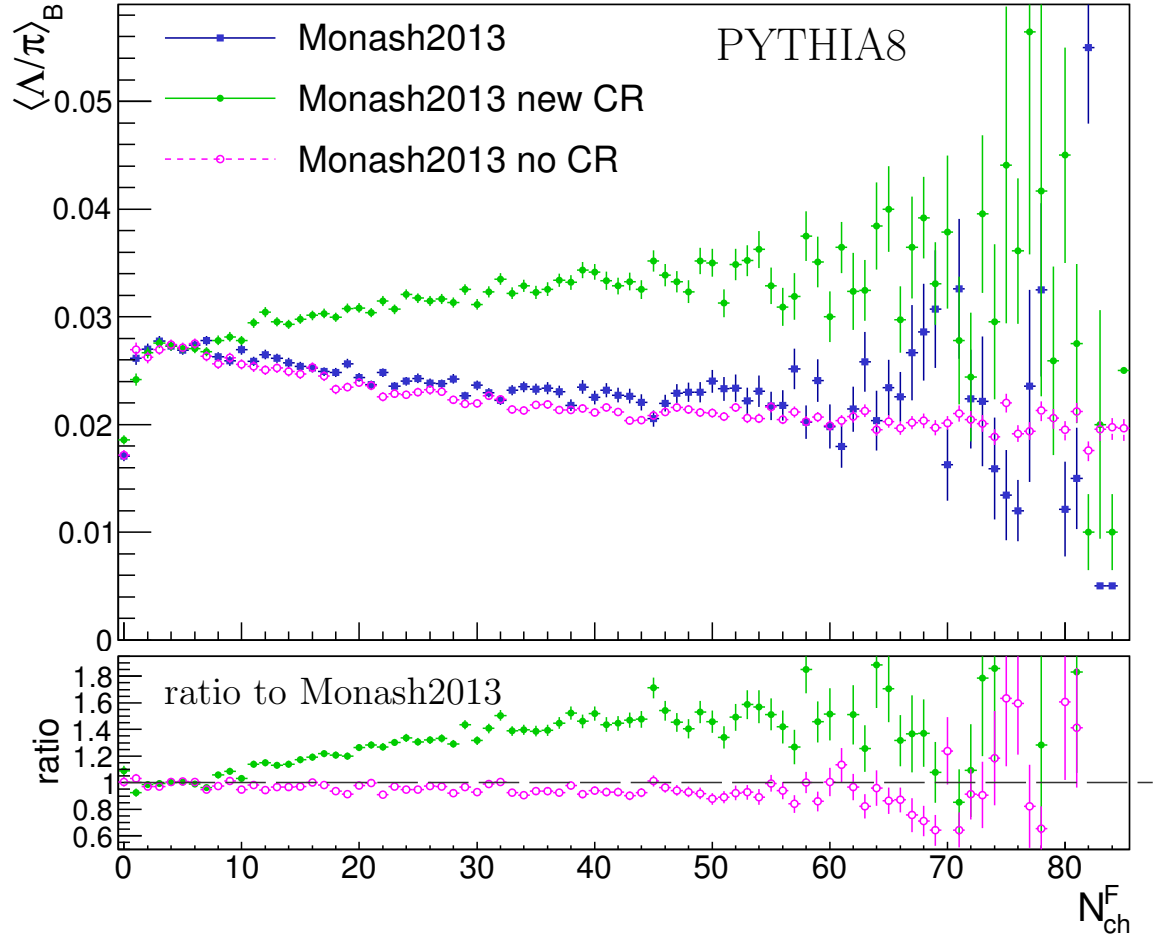

**Figure 2.** Forward-backward correlation between  $\langle \Lambda/\pi \rangle$  in backward window and  $N_{ch}$  in forward window, for three configurations of PYTHIA8 (version 8210). FB windows are  $-2.4 < \eta < -0.5$  and  $0.5 < \eta < 2.4$ .

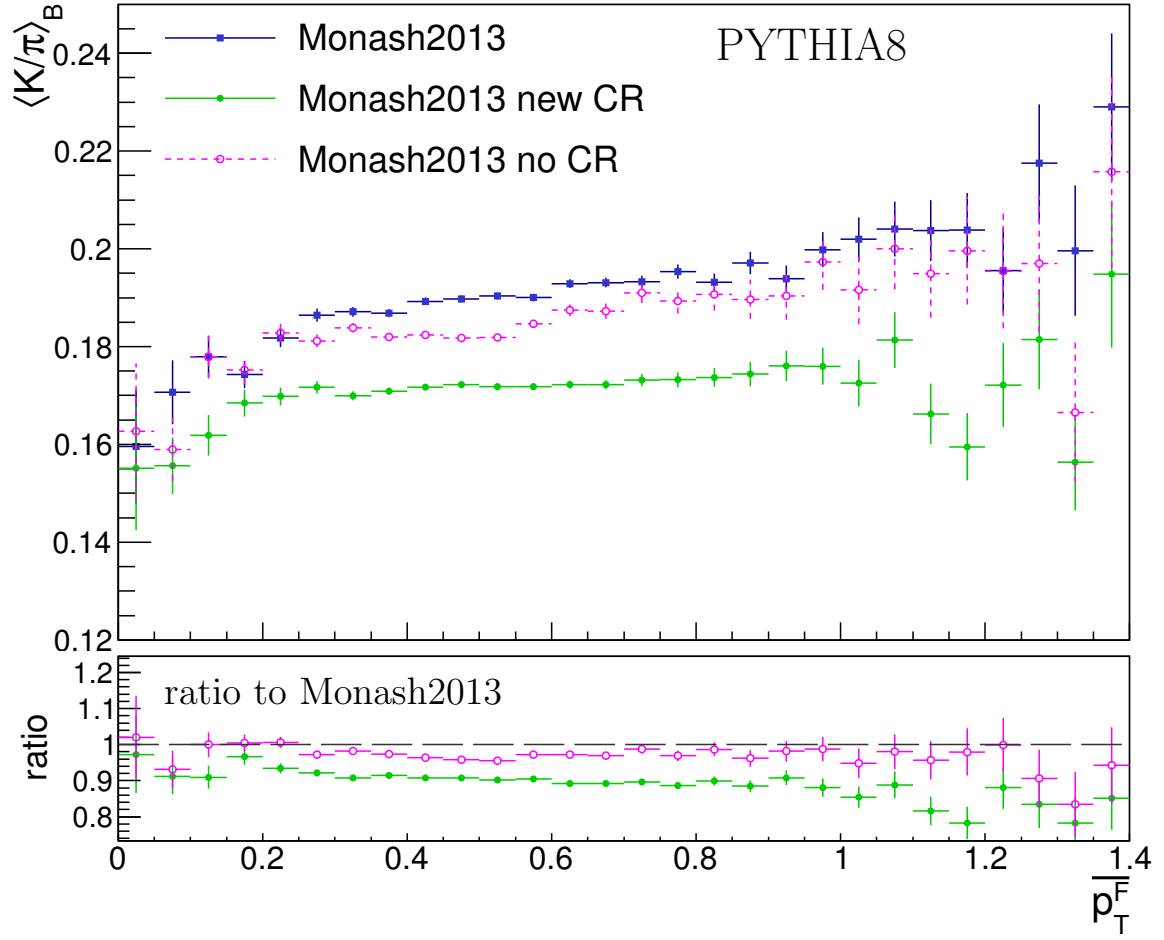

**Figure 3.** Forward-backward correlation between  $\langle K/\pi \rangle$  in backward window and  $\langle p_T \rangle$  in forward window, for three configurations of PYTHIA8 (version 8210). FB windows are  $-2.4 < \eta < -0.5$  and  $0.5 < \eta < 2.4$ .

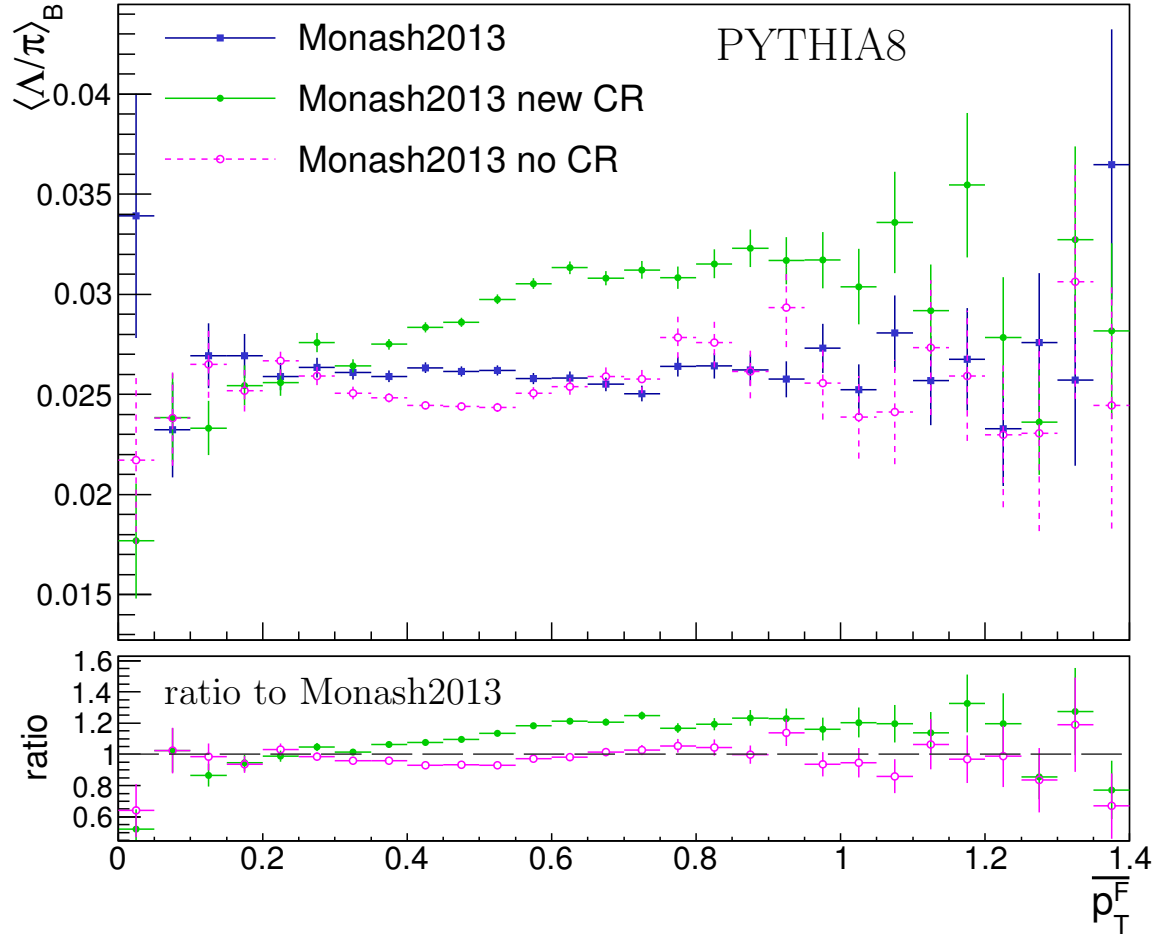

**Figure 4.** Forward-backward correlation between  $\langle \Lambda/\pi \rangle$  in backward window and  $\langle p_T \rangle$  in forward window, for three configurations of PYTHIA8 (version 8210). FB windows are  $-2.4 < \eta < -0.5$  and  $0.5 < \eta < 2.4$ .
